# Supplementary material for: The general theory of permutation equivarant neural networks and higher order graph variational encoders
Source: arXiv:2004.03990 source file (2020-04-08)
Supplement: Supplementary file 1 [file SnNN_supplement.tex]

\documentclass[11pt,reqno]{amsart}
%\pdfoutput=1
\usepackage{iclr2018_conference,times}
\usepackage{url,amsthm,amsmath,amssymb,amsfonts}
\usepackage{xcolor}
\usepackage{algorithm,algpseudocode}
\usepackage{tikz}
\usepackage{bbm}
\usepackage{rbase} 
\usepackage{paralist}
\usepackage{enumitem}
\definecolor{hcitecolor}{RGB}{40,40,160}
\usepackage[colorlinks=true,citecolor=hcitecolor, linkcolor=black]{hyperref}
\usepackage{caption}
\usepackage{subfigure}
\usepackage{graphicx}
\usepackage{pgfplots}
\usepackage{xypic}
\usepackage[all,2cell,ps,cmtip]{xy}
\usepackage{tikz}
\usepackage{caption}
\usepackage{mdframed}
\usepackage{young}
\usepackage[enableskew]{youngtab}
\Yboxdim{8pt}
\usepackage{ifthen}
%\newboolean{twocol}
%\setboolean{twocol}{false}

\newcommand{\ificml}[1]{}

\algdef{SE}[DOWHILE]{Do}{doWhile}{\algorithmicdo}[1]{\algorithmicwhile\ #1}%
\algnewcommand{\varalg}{\textit}

\usepackage{tikz}
\usetikzlibrary{shadows}
\usetikzlibrary{matrix, calc, positioning, arrows,shapes,backgrounds, arrows.meta, quotes}
\usepackage{gensymb,stmaryrd,mathtools,textcomp,xspace,grffile,rbase}

 % \mbox{}\noindent}

\ignore{
\makeatletter
\def\thm@space@setup{%
  \thm@preskip=6pt plus 0pt minus 0pt%5cm plus 1cm minus 2cm
  \thm@postskip=0pt plus 0pt minus 0pt %\thm@preskip % or whatever, if you don't want them to be equal
}
\makeatother
}

\captionsetup{width=\textwidth}
\raggedbottom

\AtBeginDocument{%
 \abovedisplayskip=6pt plus 3pt minus 3pt
 \abovedisplayshortskip=0pt plus 3pt
 \belowdisplayskip=6pt plus 3pt minus 3pt
 \belowdisplayshortskip=6pt plus 3pt minus 4pt
}

%\fancyhead[CE]{\textsc{Kondor \& Thiede}}
\fancyhead[CE]{\textsc{Permutation equivariant neural nets -- Supplement}}
\fancyhead[CO]{\textsc{Permutation equivariant neural nets -- Supplement}}

\iclrfinalcopy 

\begin{document}

\title{
The general theory of permutation equivarant neural networks}
\maketitle 
\vspace{-40pt}

\textbf{Supplementary Material}
%\\ \\ 

%\input{intro}
%\input{equivariance} 
%\input{convolutional}
%\input{fourier}
%\input{compositional} 
%\input{vae} 
% \input{experiments}
%\clearpage

\input{appendixA}
\input{appendixB}
\input{third_order_layer}
\input{further_experiments}

%\bibliography{enn}
%\bibliographystyle{iclr2018_conference}

\end{document}
